# Supplementary material for: Chiral Phonons Arising From Chirality-Selective Magnon-Phonon Coupling
Source: arXiv:2411.03879 source file (2025-11-18)
Supplement: Supplementary file 1 [file SM_Truly_Chiral_Phonons_Arising_From_Chirality_Selective_Magnon_Phonon_Coupling.pdf]

# Supplemental Material: Truly Chiral Phonons Arising From Chirality-Selective Magnon-Phonon Coupling

Markus Weißenhofer,<sup>1,2,\*</sup> Philipp Rieger,<sup>1</sup> M. S. Mrudul,<sup>3</sup> Luca Mikadze,<sup>1</sup> Ulrich Nowak,<sup>4</sup> and Peter M. Oppeneer<sup>1</sup>

<sup>1</sup>*Department of Physics and Astronomy, Uppsala University, P. O. Box 516, S-751 20 Uppsala, Sweden*

<sup>2</sup>*Department of Physics, Freie Universität Berlin, Arnimallee 14, D-14195 Berlin, Germany*

<sup>3</sup>*Department of Physics and Astronomy, Uppsala University, P. O. Box 516, S-751 20 Uppsala, Sweden*

<sup>4</sup>*Department of Physics, University of Konstanz, DE-78457 Konstanz, Germany*

(Dated: November 6, 2024)

## I. DERIVATION OF MAGNON-PHONON HAMILTONIAN

In this section, we derive the magnon-phonon Hamiltonian up to second order in operators from the atomistic spin-lattice Hamiltonian discussed in the main part,

$$\hat{\mathcal{H}}_{\text{SLC}} = \sum_i \frac{\hat{\mathbf{P}}_i^2}{2m} + \sum_{ij,\alpha\beta} \left( \Phi_{ij}^{\alpha\beta} \hat{X}_i^\alpha \hat{X}_j^\beta + J_{ij}^{\alpha\beta} \hat{S}_i^\alpha \hat{S}_j^\beta \right) + \sum_{ijk,\alpha\beta\gamma} \left( J_{ijk}^{\alpha\beta\gamma} \hat{S}_i^\alpha \hat{S}_j^\beta \hat{X}_k^\gamma + G_{ijk}^{\alpha\beta\gamma} \hat{S}_i^\alpha \hat{X}_j^\beta \hat{P}_k^\gamma \right). \quad (1)$$

As a first step, we express position, momentum, and spin operators by Fourier transforms,

$$\hat{X}_i^\alpha = \frac{1}{\sqrt{N}} \sum_{\mathbf{k}} e^{i\mathbf{k}\cdot\mathbf{r}_i} \hat{X}_{\mathbf{k}}^\alpha, \quad \hat{P}_i^\alpha = \frac{1}{\sqrt{N}} \sum_{\mathbf{k}} e^{i\mathbf{k}\cdot\mathbf{r}_i} \hat{P}_{\mathbf{k}}^\alpha, \quad \hat{S}_i^\alpha = \frac{1}{\sqrt{N}} \sum_{\mathbf{k}} e^{i\mathbf{k}\cdot\mathbf{r}_i} \hat{S}_{\mathbf{k}}^\alpha, \quad (2)$$

$$\hat{X}_{\mathbf{k}}^\alpha = \frac{1}{\sqrt{N}} \sum_i e^{-i\mathbf{k}\cdot\mathbf{r}_i} \hat{X}_i^\alpha, \quad \hat{P}_{\mathbf{k}}^\alpha = \frac{1}{\sqrt{N}} \sum_i e^{-i\mathbf{k}\cdot\mathbf{r}_i} \hat{P}_i^\alpha, \quad \hat{S}_{\mathbf{k}}^\alpha = \frac{1}{\sqrt{N}} \sum_i e^{-i\mathbf{k}\cdot\mathbf{r}_i} \hat{S}_i^\alpha. \quad (3)$$

Inserting these into Eq. (1) yields

$$\begin{aligned} \hat{\mathcal{H}}_{\text{SLC}} = & \frac{1}{2m} \sum_{\mathbf{k}\alpha} \hat{P}_{\mathbf{k}}^\alpha \hat{P}_{-\mathbf{k}}^\alpha + \sum_{\mathbf{k}\alpha\beta} \left( m \mathcal{D}_{\mathbf{k}}^{\alpha\beta} \hat{X}_{\mathbf{k}}^\alpha \hat{X}_{-\mathbf{k}}^\beta + \tilde{J}_{\mathbf{k}}^{\alpha\beta} \hat{S}_{\mathbf{k}}^\alpha \hat{S}_{-\mathbf{k}}^\beta \right) \\ & + \frac{1}{\sqrt{N}} \sum_{\mathbf{k}\mathbf{k}',\alpha\beta\gamma} \left( \tilde{J}_{\mathbf{k}',-\mathbf{k}-\mathbf{k}'}^{\alpha\beta\gamma} \hat{S}_{\mathbf{k}}^\alpha \hat{S}_{\mathbf{k}'}^\beta \hat{X}_{-\mathbf{k}-\mathbf{k}'}^\gamma + \tilde{G}_{\mathbf{k}',-\mathbf{k}-\mathbf{k}'}^{\alpha\beta\gamma} \hat{S}_{\mathbf{k}}^\alpha \hat{X}_{\mathbf{k}'}^\beta \hat{P}_{-\mathbf{k}-\mathbf{k}'}^\gamma \right), \end{aligned} \quad (4)$$

where we have used the orthogonality relation  $\frac{1}{N} \sum_i e^{i\mathbf{k}-\mathbf{k}'\cdot\mathbf{r}_i} = \delta_{\mathbf{k},\mathbf{k}'}$  and introduced the following quantities

$$\begin{aligned} \mathcal{D}_{\mathbf{k}}^{\alpha\beta} &= \frac{1}{m} \sum_j \Phi_{ij}^{\alpha\beta} e^{-i\mathbf{k}\cdot(\mathbf{r}_j-\mathbf{r}_i)}, \quad \tilde{J}_{\mathbf{k}}^{\alpha\beta} = \sum_j J_{ij}^{\alpha\beta} e^{-i\mathbf{k}\cdot(\mathbf{r}_j-\mathbf{r}_i)}, \\ \tilde{J}_{\mathbf{k}\mathbf{k}'}^{\alpha\beta\gamma} &= \sum_{jk} e^{i\mathbf{k}\cdot(\mathbf{r}_j-\mathbf{r}_i)} e^{i\mathbf{k}'\cdot(\mathbf{r}_k-\mathbf{r}_i)} J_{ijk}^{\alpha\beta\gamma}, \quad \tilde{G}_{\mathbf{k}\mathbf{k}'}^{\alpha\beta\gamma} = \sum_{jk} e^{i\mathbf{k}\cdot(\mathbf{r}_j-\mathbf{r}_i)} e^{i\mathbf{k}'\cdot(\mathbf{r}_k-\mathbf{r}_i)} G_{ijk}^{\alpha\beta\gamma}. \end{aligned} \quad (5)$$

Next, we use the Holstein-Primakoff transformation [1] to describe magnon excitations in the fully spin-polarized configuration along  $z$ . For this purpose, spin raising and lowering operators are defined as  $\hat{S}_i^\pm = \hat{S}_i^x \pm i\hat{S}_i^y$ . The resulting Holstein-Primakoff transformation can be written as

$$\hat{S}_i^+ = \sqrt{2S - \hat{b}_i^\dagger \hat{b}_i} \hat{b}_i, \quad \hat{S}_i^- = \hat{b}_i^\dagger \sqrt{2S - \hat{b}_i^\dagger \hat{b}_i}, \quad \hat{S}_i^z = S - \hat{b}_i^\dagger \hat{b}_i, \quad (6)$$

with  $\hat{b}_i^{(\dagger)}$  being bosonic annihilation (creation) operators. The square roots can be expanded in terms of  $\hat{b}_i^\dagger \hat{b}_i / (2S)$ , yielding a series  $\sqrt{2S - \hat{b}_i^\dagger \hat{b}_i} = \sqrt{2S} [1 - \hat{b}_i^\dagger \hat{b}_i / (4S) + \dots]$ . Here, we only want to keep terms up to second order in

---

\* markus.weissenhofer@fu-berlin.de

operators in the final Hamiltonian. Thus, omitting all terms above the zeroth order in the expansion of the square root is sufficient. Introducing Fourier transforms of the bosonic operators,

$$\hat{b}_i = \frac{1}{\sqrt{N}} \sum_{\mathbf{k}} e^{i\mathbf{k} \cdot \mathbf{r}_i} \hat{b}_{\mathbf{k}}, \quad \hat{b}_i^\dagger = \frac{1}{\sqrt{N}} \sum_{\mathbf{k}} e^{-i\mathbf{k} \cdot \mathbf{r}_i} \hat{b}_{\mathbf{k}}^\dagger, \quad (7)$$

$$\hat{b}_{\mathbf{k}} = \frac{1}{\sqrt{N}} \sum_i e^{-i\mathbf{k} \cdot \mathbf{r}_i} \hat{b}_i, \quad \hat{b}_{\mathbf{k}}^\dagger = \frac{1}{\sqrt{N}} \sum_i e^{i\mathbf{k} \cdot \mathbf{r}_i} \hat{b}_i^\dagger, \quad (8)$$

we can write the Fourier transformed spin operators up to second order in bosonic operators as

$$\hat{S}_{\mathbf{k}}^x = \frac{\sqrt{S}}{\sqrt{2}} (\hat{b}_{\mathbf{k}} + \hat{b}_{-\mathbf{k}}^\dagger), \quad \hat{S}_{\mathbf{k}}^y = -i \frac{\sqrt{S}}{\sqrt{2}} (\hat{b}_{\mathbf{k}} - \hat{b}_{-\mathbf{k}}^\dagger), \quad \hat{S}_{\mathbf{k}}^z = S\sqrt{N} \delta_{\mathbf{k},0} - \frac{1}{\sqrt{N}} \sum_{\mathbf{k}'} \hat{b}_{\mathbf{k}'}^\dagger \hat{b}_{\mathbf{k}+\mathbf{k}'}. \quad (9)$$

In addition, we perform the usual normal mode expansion of the lattice operators,

$$\hat{X}_{\mathbf{k}}^\alpha = \sum_{\lambda} \sqrt{\frac{\hbar}{2m\omega_{\mathbf{k}\lambda}}} \chi_{\mathbf{k}\lambda}^\alpha (\hat{a}_{\mathbf{k}\lambda} + \hat{a}_{-\mathbf{k}\lambda}^\dagger), \quad \hat{P}_{\mathbf{k}}^\alpha = -i \sum_{\lambda} \sqrt{\frac{\hbar m \omega_{\mathbf{k}\lambda}}{2}} \chi_{\mathbf{k}\lambda}^\alpha (\hat{a}_{\mathbf{k}\lambda} - \hat{a}_{-\mathbf{k}\lambda}^\dagger), \quad (10)$$

with  $\omega_{\mathbf{k}\lambda}^2$  and  $\chi_{\mathbf{k}\lambda}^\alpha$  being the  $\lambda$ -th eigenvalue and eigenvector of the dynamical matrix  $\mathcal{D}_{\mathbf{k}}$  and where  $\hat{a}_{\mathbf{k}\lambda}^{(\dagger)}$  are phonon annihilation (creation) operators.

Inserting the expressions for  $\hat{X}_{\mathbf{k}}^\alpha$ ,  $\hat{P}_{\mathbf{k}}^\alpha$ , and  $\hat{S}_{\mathbf{k}}^\alpha$  into Eq. (11), together with the spectral decomposition of the dynamical matrix  $\mathcal{D}_{\mathbf{k}}^{\alpha\beta} = \sum_{\lambda} \omega_{\mathbf{k}\lambda}^2 \chi_{\mathbf{k}\lambda}^\alpha (\chi_{\mathbf{k}\lambda}^\beta)^*$ , we obtain up to second order in operators

$$\begin{aligned} \hat{\mathcal{H}}_{\text{SLC}} = & \sum_{\mathbf{k}\lambda} \hbar \omega_{\mathbf{k}\lambda} \hat{a}_{\mathbf{k}\lambda}^\dagger \hat{a}_{\mathbf{k}\lambda} + \sum_{\mathbf{k}} \varepsilon_{\mathbf{k}} \hat{b}_{\mathbf{k}}^\dagger \hat{b}_{\mathbf{k}} \\ & + \sum_{\mathbf{k}\lambda} (c_{\mathbf{k}\lambda}^- \hat{b}_{-\mathbf{k}} + c_{\mathbf{k}\lambda}^+ \hat{b}_{\mathbf{k}}^\dagger) (\hat{a}_{\mathbf{k}\lambda} + \hat{a}_{-\mathbf{k}}^\dagger) + \sum_{\mathbf{k}\lambda\lambda'} g_{\mathbf{k}\lambda\lambda'} (\hat{a}_{\mathbf{k}\lambda} + \hat{a}_{-\mathbf{k}\lambda}^\dagger) (\hat{a}_{-\mathbf{k}\lambda'} - \hat{a}_{\mathbf{k}\lambda'}^\dagger). \end{aligned} \quad (11)$$

Here we have neglected zero-point energies and used that  $\sum_{\mathbf{k}} J_{ij}^{\alpha\beta\gamma} = 0$ . The latter is generally required for translational invariance of the Hamiltonian [2] and we have shown it to be fulfilled for bcc Fe in particular.

The magnon energies  $\varepsilon_{\mathbf{k}}$  depend on the specific interactions included in the exchange couplings  $J_{ij}^{\alpha\beta}$ . Considering only isotropic Heisenberg exchange and on-site uniaxial magneto-crystalline anisotropy along  $z$ , we can write  $J_{ij}^{\alpha\beta} = \delta_{ij} \delta^{\alpha z} \delta^{\beta z} d_z + (1 - \delta_{ij}) \delta^{\alpha\beta} J_{ij}$  and the magnon energies read

$$\varepsilon_{\mathbf{k}} = S \left( 2d_z + 2 \sum_j J_{ij} \left[ 1 - e^{-i\mathbf{k} \cdot (\mathbf{r}_j - \mathbf{r}_i)} \right] \right). \quad (12)$$

Furthermore, in Eq. (11) we have introduced magnon-phonon and phonon-phonon coupling parameters as

$$c_{\mathbf{k}\lambda}^\pm = \sqrt{\frac{\hbar S^3}{m \omega_{\mathbf{k}\lambda}}} \sum_{\gamma} (\tilde{J}_{0\mathbf{k}}^{xz\gamma} \pm i \tilde{J}_{0\mathbf{k}}^{yz\gamma}) \chi_{\mathbf{k}\lambda}^\gamma, \quad (13)$$

$$g_{\mathbf{k}\lambda\lambda'} = -\frac{i\hbar S}{2} \sqrt{\frac{\omega_{\mathbf{k}\lambda'}}{\omega_{\mathbf{k}\lambda}}} \sum_{\beta\gamma} \tilde{G}_{\mathbf{k},-\mathbf{k}}^{z\beta\gamma} \chi_{\mathbf{k}\lambda}^\beta (\chi_{\mathbf{k}\lambda'}^\gamma)^*. \quad (14)$$

## II. BARE BANDSTRUCTURES

In this section we show the bare phonon [Fig. S1(a)] and magnon bands [Fig. S1(b)], i.e., the bands in the absence of spin-lattice coupling.

The bare phonon frequencies and polarization vectors were calculated using spin-polarized density functional theory in the local density approximation. Specifically, we have used the density-functional perturbation theory implementation of Quantum ESPRESSO [3, 4] using an experimental lattice constant of  $a = 2.8665 \text{ \AA}$ .

The magnons are obtained from the expression for the magnon energy derived above, *viz.*

$$\varepsilon_{\mathbf{k}} = S \left( 2d_z + 2 \sum_j J_{ij} \left[ 1 - e^{-i\mathbf{k} \cdot (\mathbf{r}_j - \mathbf{r}_i)} \right] \right), \quad (15)$$

which we evaluate using first-principles exchange constants  $J_{ij}$  [5] (summarized in Table SI) and a magneto-crystalline energy taken from experimental measurements [6]. Note that we have to scale the parameters, due to a contrasting convention used in the Heisenberg Hamiltonian: here, we use  $\mathcal{H}_H = \sum_{ij} J_{ij} \hat{\mathbf{S}}_i \cdot \hat{\mathbf{S}}_j$  with  $|\hat{\mathbf{S}}_i| = S$ , while in Ref. [5], the Heisenberg Hamiltonian is written as  $\mathcal{H}_H = \sum_{ij} J'_{ij} \hat{\mathbf{e}}_i \cdot \hat{\mathbf{e}}_j$ , with  $\hat{\mathbf{e}}_i = \hat{\mathbf{S}}_i/|S|$  being unit vectors. One immediately sees that  $J_{ij} = J'_{ij}/S^2$ . Similarly, we have to rescale the experimental value for the magneto-crystalline energy, i.e.,  $d/S^2 = 6.97 \text{ \mu eV}$  [6].

For bcc Fe we get that  $S = \mu_s/(g\mu_B) \approx 1.1$  [7], with a spin  $g$ -factor of approximately two.

Table SI. *Ab initio* calculated Heisenberg exchange constants for bcc Fe as a function of neighboring shell, taken from Ref. [5].

| Shell   | $J'_{ij}$ (mRy) |
|---------|-----------------|
| First   | 1.200           |
| Second  | 0.646           |
| Third   | 0.007           |
| Fourth  | -0.108          |
| Fifth   | -0.071          |
| Sixth   | 0.035           |
| Seventh | 0.002           |
| Eighth  | 0.014           |

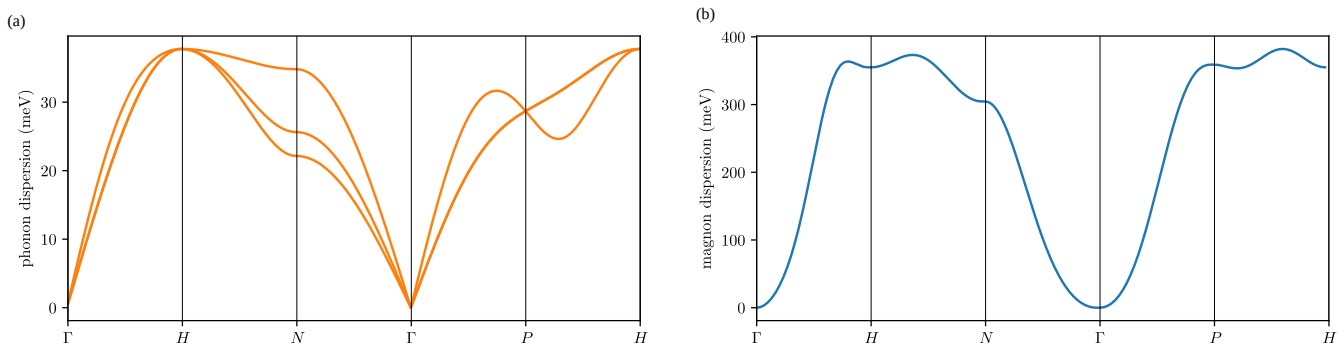

Figure S1. Calculated bare phonon (a) and magnon dispersions (b) of ferromagnetic bcc Fe along high-symmetry lines.

### III. PHONON ANGULAR MOMENTUM AND CHIRALITY IN VARIOUS PLANES IN THE BRILLOUIN ZONE

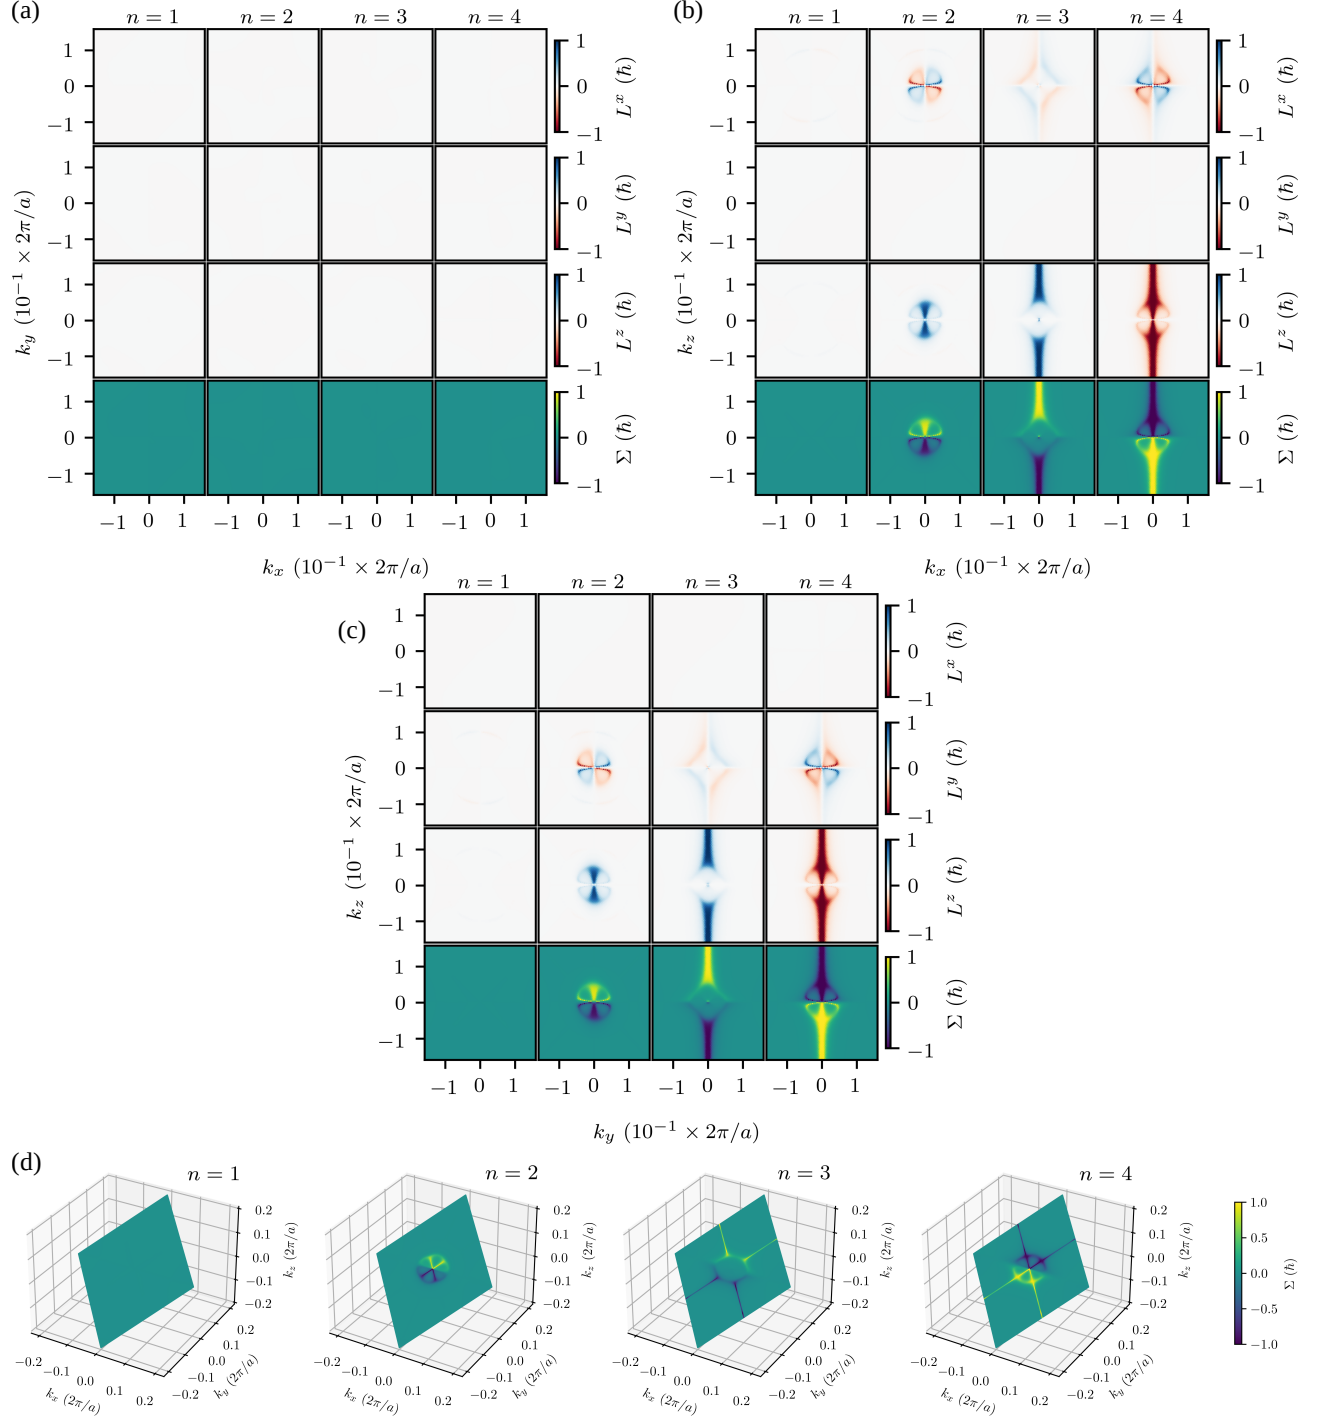

Figure S2. Phonon angular momentum  $\mathbf{L}$  and phonon chirality  $\Sigma = \mathbf{L} \cdot \mathbf{v}/|\mathbf{v}|$  of the coupled magnon-phonon bands for bcc Fe in (a) the  $k_x$ - $k_y$  plane, (b) the  $k_x$ - $k_z$  plane, (c) the  $k_y$ - $k_z$  plane, and (d) a diagonal plane orthogonal to the  $(0, -1, 1)$  direction in  $\mathbf{k}$  space. The index  $n$  labels the magnon-phonon modes:  $n = 1$  is the longitudinal acoustic phonon that does not couple to magnons at all,  $n = 4$  is the transverse acoustic phonon without avoided crossing and  $n = 2, 3$  are the two magnon-polaron bands.

- 
- [1] T. Holstein and H. Primakoff, Field Dependence of the Intrinsic Domain Magnetization of a Ferromagnet, *Phys. Rev.* **58**, 1098 (1940).
  - [2] J. Hellsvik, D. Thonig, K. Modin, D. Iuşan, A. Bergman, O. Eriksson, L. Bergqvist, and A. Delin, General method for atomistic spin-lattice dynamics with first-principles accuracy, *Phys. Rev. B* **99**, 104302 (2019).
  - [3] P. Giannozzi, S. Baroni, N. Bonini, M. Calandra, R. Car, C. Cavazzoni, D. Ceresoli, G. L. Chiarotti, M. Cococcioni, I. Dabo, A. D. Corso, S. de Gironcoli, S. Fabris, G. Fratesi, R. Gebauer, U. Gerstmann, C. Gougoussis, A. Kokalj, M. Lazzeri, L. Martin-Samos, N. Marzari, F. Mauri, R. Mazzarello, S. Paolini, A. Pasquarello, L. Paulatto, C. Sbraccia, S. Scandolo, G. Sclauzero, A. P. Seitsonen, A. Smogunov, P. Umari, and R. M. Wentzcovitch, QUANTUM ESPRESSO: a modular and open-source software project for quantum simulations of materials, *J. Phys.: Condens. Matter* **21**, 395502 (2009).
  - [4] P. Giannozzi, O. Andreussi, T. Brumme, O. Bunau, M. B. Nardelli, M. Calandra, R. Car, C. Cavazzoni, D. Ceresoli, M. Cococcioni, N. Colonna, I. Carnimeo, A. D. Corso, S. de Gironcoli, P. Delugas, R. A. DiStasio, A. Ferretti, A. Floris, G. Fratesi, G. Fugallo, R. Gebauer, U. Gerstmann, F. Giustino, T. Gorni, J. Jia, M. Kawamura, H.-Y. Ko, A. Kokalj, E. Küçükbenli, M. Lazzeri, M. Marsili, N. Marzari, F. Mauri, N. L. Nguyen, H.-V. Nguyen, A. O. de-la Roza, L. Paulatto, S. Poncé, D. Rocca, R. Sabatini, B. Santra, M. Schlipf, A. P. Seitsonen, A. Smogunov, I. Timrov, T. Thonhauser, P. Umari, N. Vast, X. Wu, and S. Baroni, Advanced capabilities for materials modelling with Quantum ESPRESSO, *J. Phys.: Condens. Matter* **29**, 465901 (2017).
  - [5] O. N. Mryasov, A. J. Freeman, and A. I. Liechtenstein, Theory of non-Heisenberg exchange: Results for localized and itinerant magnets, *J. Appl. Phys.* **79**, 4805 (1996).
  - [6] I. Razdolski, A. Alekhin, N. Ilin, J. P. Meyburg, V. Roddatis, D. Diesing, U. Bovensiepen, and A. Melnikov, Nanoscale interface confinement of ultrafast spin transfer torque driving non-uniform spin dynamics, *Nature Commun.* **8**, 15007 (2017).
  - [7] R. F. L. Evans, W. J. Fan, P. Chureemart, T. A. Ostler, M. O. A. Ellis, and R. W. Chantrell, Atomistic spin model simulations of magnetic nanomaterials, *J. Phys.: Condens. Matter* **26**, 103202 (2014).
